# Supplementary material for: Interpretable Image Classification via Non-parametric Part Prototype Learning
Source: arXiv:2503.10247 source file (2025-03-13)
Supplement: Supplementary file 1 [file X_suppl.tex]

\clearpage
\appendix
\maketitlesupplementary

\setcounter{page}{1}
\setcounter{section}{0}
\setcounter{table}{0}
\setcounter{figure}{0}

This document provides more implementation and experimental details of our framework, as well as more quantitative and qualitative results:
\begin{itemize}
  \item Section \ref{sec:supp-details} provides more implementation details
  \item Section \ref{sec:supp-experimental-details} describes additional details on experiments
  \item Section \ref{sec:supp-results} provides more experimental results
  \item Section \ref{sec:supp-visualizations} provides additional visualizations in comparison with previous works
\end{itemize}
\section{Implementation Details}
\label{sec:supp-details}

\noindent During the first stage of training, given the patch tokens $\mathbf{f} \in \mathbb{R}^{Bhw \times D}$ that encodes a batch of images, the foreground extraction module $\phi$ estimates a binary mask $\mathcal{M} \in \{0,1\}^{Bhw}$ where a value of $1$ indicates that the corresponding patch token is in the foreground of the input image it belongs to. With this, the patch tokens $\mathbf{f}^c$ that belongs to each class $c$ in a batch of training samples can be defined as:

\begin{equation*}
  \mathbf{f}^c := \{ \mathbf{f}_i \mid \mathcal{M}_i=1, \mathcal{Y}_i=c\},
\end{equation*}

where $\mathcal{Y} \in \{c_1, c_2, ...\}^{Bhw}$ denotes the class label of the input image that each patch token belongs to. The foreground extractor $\phi$ can be implemented using various off-the-shelf methods, such as PaPr \cite{mahmud_papr_2024}, Principle Component Analysis \cite{oquab_dinov2_2024} and Attention Rollout \cite{xue_protopformer_2022}. We ablate these methods in Table \ref{tab:ablation-fg-extraction}. In addition, we adopt cosine similarity to compute similarity $\mathbf{S}$ between the patch tokens $\mathbf{f}$ and prototypes $\mathbf{P}$:

\begin{equation*}
  \mathbf{S} = \frac{\mathbf{f}^{\top}\mathbf{P}}{\left\lVert \mathbf{f} \right\lVert_2 \left\lVert \mathbf{P} \right\lVert_2}.
\end{equation*}

\noindent During the first stage of training, we initialize the prototypes from $\mathcal{N}(0.0, 0.02)$ and the modulation weights with $w^c_k=0.2$. We provide an overview of our training procedure in Algorithm \ref{alg:training}. When adapting to concept learning, we construct the concept bottleneck layer by replacing the modulation weights $w$ with two fully connected layers, where the output dimension of the first layer equal to the number of concepts associated with all classes.

\noindent \textbf{Distinctiveness and Comprehensiveness Scores.} The calculation of Comprehensiveness Score requires the ground truth foreground masks of test images, while the calculation of Distinctiveness Score is label-free. We provide Python-like pseudo-code for calculating these two scores in Algorithm \ref{alg:distinctiveness} and Algorithm \ref{alg:compre}.

\begin{algorithm}
\caption{Prototype Learning and Backbone Fine-tuning}
\label{alg:training}
\begin{algorithmic}[1]
  \Require Training set $\mathcal{X}$, $nEpochs$, ViT backbone $\mathcal{F}$
\State Initialize prototypes $\mathbf{P}$ and modulation vector $w$ with $\mathbf{P} \sim \mathcal{N}(0.0, 0.02)$ and $w^c_k=0.2$
\For{$t \in \{1, \dots, nEpochs\}$}
    \State Randomly split $\mathcal{X}$ into mini-batches
    \For{$(\mathbf{X}, \mathbf{y}) \in \{\mathcal{X}_1, \dots\}$}
        \State $\mathbf{f} = \text{reshape}(\mathcal{F}(\mathbf{X})) \in \mathbb{R}^{Bhw \times D}$
        \State $\mathcal{M} = \phi(\mathbf{f}, \mathbf{X}) \in \{0, 1\}^{Bhw}$
        \State $\mathbf{S} = \text{reshape}(\text{Sim}(\mathbf{f}, \mathbf{P})) \in \mathbb{R}^{Bhw \times N \times K}$
        \For{$c \in \text{unique}(\mathbf{y})$}
          \State Get $\mathbf{S}^c$ and $\mathbf{f}^c$ by indexing $\mathbf{S}$, $\mathbf{f}$ with $\mathcal{M}$, $\mathbf{y}$
          \State $\mathbf{A}^{c,*} = \text{sinkhorn\_knopp}(\mathbf{S}^c)$
          \If{\textit{first training stage}}
            \State $\mathbf{P}^c \leftarrow \beta \mathbf{P}^c + (1 - \beta) (\mathbf{A}^{c,*})^\top\mathbf{f}^c$
          \EndIf
        \EndFor
        \State $g = \text{MaxPool}(\text{reshape}(\mathbf{S})) \in \mathbb{R}^{N \times K}$
        \State $\text{logits} = \text{compute\_logits}(g, w) \in \mathbb{R}^N$
        \If{\textit{second training stage}}
          \State Compute loss $\mathcal{L}_{xe}(\text{logits}, \mathbf{y})$
          \State Compute loss $\mathcal{L}_{PPC}(\mathbf{S}, \mathbf{A})$
          \State Minimize loss by updating $\mathcal{F}$
        \EndIf
    \EndFor
\EndFor
\end{algorithmic}
\end{algorithm}

\section{Experimental Details}
\label{sec:supp-experimental-details}

\noindent \textbf{Implementations.} We train our network with a batch size of 128 and input size of 224. For experiments on all three datasets, We trained previous Prototypical-Part Networks by setting the number of part prototypes per class $K=\{3,5\}$, and the number of added Vision Transformer blocks $m=3$. Specifically, each identity block is copied from the 4th, 8th and 12th Transformer blocks in the original sequence, with the weights of attention projection layer and the second fully-connected layer set of zero, each inserted after the block they are copied from. We use a learning rate of $1e-4$ to train these blocks while freezing the rest of the backbone during the joint learning phase of these methods. All the other hyperparameters are the same as the ones in original implementations.

\noindent \textbf{Datasets.} CUB-200-2011 contains keypoint annotation of 15 parts and foreground segmentation masks for each image besides image-level class levels, which are used to calculate the Consistency score proposed in \cite{huang_evaluation_2023} and our Comprehensiveness score. We followed ProtoPNet \cite{chen_this_2019} to perform offline data augmentation when training each method. Each image is augmented 40 times with random rotation, random skew, random shear and horizontal flip. For evaluation on Stanford Cars and Stanford Dogs, we did not perform any additional data augmentation besides resizing.

\section{Additional Results}
\label{sec:supp-results}

The results on Stanford Cars and Stanford Dogs datasets over two backbones are shown in Table \ref{tab:supp-cars-results} and Table \ref{tab:supp-dogs-results}.

\newcolumntype{Y}{>{\centering\arraybackslash}X}

\begin{table}
  \centering
  \resizebox{0.95\columnwidth}{!}{
  \begin{tabularx}{\columnwidth}{c|Y|Y}
    \toprule
      \textbf{Methods} & \textbf{ViT-B} & \textbf{ViT-S} \\
      \midrule
      ProtoPNet (K=3) & 86.47 & 78.16 \\
      ProtoPNet (K=5) & 86.75 & 79.51 \\
      \hline
      TesNet (K=3) & 87.33 & 80.97 \\
      TesNet (K=5) & 87.15 & 82.55 \\
      \hline
      EvalProtoPNet & 91.20 & 83.40 \\
      EvalProtoPNet & 91.46 & \textbf{87.09} \\
      \hline
      Ours (K=3) & 91.29 & 85.52 \\
      Ours (K=5) & \textbf{93.63} & 86.10 \\
      \bottomrule
    \end{tabularx}
  }
  \caption{Classification results on Stanford Cars dataset. All methods are trained with DINOv2. Best results are in bold.}
  \label{tab:supp-cars-results}
\end{table}

\newcolumntype{Y}{>{\centering\arraybackslash}X}

\begin{table}
  \centering
  \resizebox{0.95\columnwidth}{!}{
  \begin{tabularx}{\columnwidth}{c|Y|Y}
    \toprule
      \textbf{Methods} & \textbf{ViT-B} & \textbf{ViT-S} \\
      \midrule
      ProtoPNet (K=3) & 84.11 & 79.25 \\
      ProtoPNet (K=5) & 84.90 & 79.28 \\
      \hline
      TesNet (K=3) & 85.16 & 82.14 \\
      TesNet (K=5) & 87.44 & 82.01 \\
      \hline
      EvalProtoPNet & 87.88 & 83.68 \\
      EvalProtoPNet & 88.08 & 83.80 \\
      \hline
      Ours (K=3) & 87.05 & 83.11 \\
      Ours (K=5) & \textbf{88.59} & \textbf{83.93} \\
      \bottomrule
    \end{tabularx}
  }
  \caption{Classification results on Stanford Dogs dataset. All methods are trained with DINOv2. Best results are in bold.}
  \label{tab:supp-dogs-results}
\end{table}

\noindent \textbf{Foreground Extraction.} We experimented with a few methods that can be directly used with our framework. PaPr \cite{mahmud_papr_2024} produces a foreground mask by thresholding the feature map from the last layer of a lightweight convolutional backbone such as resnet18 and MobileNets. Attention Rollout \cite{xue_protopformer_2022} calculates the foreground mask with the attention values between the patch tokens and the \texttt{cls} token of each Transformer block of a ViT backbone. Finally, the foreground masks can also be obtained by thresholding the first principal component of a batch of patch tokens \cite{oquab_dinov2_2024}. Table \ref{tab:ablation-fg-extraction} shows the effect of each method on the performance of our framework.

\begin{table}[b]
  \centering
  \resizebox{\columnwidth}{!}{
    \begin{tabular}{lcccc}
      \toprule
      & Con. & Sta. & Dis. & Class. \\
      \hline
      No foreground extraction & 29.67 & 82.85 & 94.17 & 88.42 \\
      PaPr w/ resnet18 & 51.01 & 82.33 & 97.23 & 88.76 \\
      Attention Rollout & 61.90 & 79.97 & 92.77 & 90.75 \\
      First Principal Component & \textbf{66.40} & \textbf{82.97} & \textbf{94.45} & \textbf{90.82} \\
      \bottomrule
    \end{tabular}
  }
  \caption{The effect of various off-the-shelf ViT foreground patch extraction methods on the performance of our framework.}
  \label{tab:ablation-fg-extraction}
\end{table}

\begin{algorithm}[t]
  \caption{Python-like pseudo-code of Distinctiveness Score calculation.}
  \label{alg:distinctiveness}
  \definecolor{codeblue}{rgb}{0.25,0.5,0.5}
  \lstset{
    backgroundcolor=\color{white},
    basicstyle=\fontsize{6pt}{6pt}\ttfamily\selectfont,
    columns=fullflexible,
    breaklines=true,
    captionpos=b,
    commentstyle=\fontsize{6pt}{6pt}\color{codeblue},
    keywordstyle=\fontsize{6pt}{6pt},
  }
\begin{lstlisting}[language=python]
def evaluate_distinctiveness(model, test_dataset, bbox_size):
    all_O_x = []
    for image in test_dataset:
        activations = model.get_activation(images) # shape: K, H, W
        sample_IoUs = []
        for i in range(K):
            for j in range(K):
                activation_i_max_coord = max_coord(activations[i])
                activation_j_max_coord = max_coord(activations[j])
                bbox_i = get_bbox(activation_i_max_coord)
                bbox_j = get_bbox(activation_j_max_coord)
                IoU = compute_box_IoU(bbox_i, bbox_j)
                sample_IoUs.append(IoU)
        O_x = mean(sample_IoUs)
        all_O_x.append(O_x)
    return 1 - mean(all_O_x)
\end{lstlisting}
\end{algorithm}

\begin{algorithm}[t]
  \caption{Python-like pseudo-code of Comprehensiveness Score calculation.}
  \label{alg:compre}
  \definecolor{codeblue}{rgb}{0.25,0.5,0.5}
  \lstset{
    backgroundcolor=\color{white},
    basicstyle=\fontsize{6pt}{6pt}\ttfamily\selectfont,
    columns=fullflexible,
    breaklines=true,
    captionpos=b,
    commentstyle=\fontsize{6pt}{6pt}\color{codeblue},
    keywordstyle=\fontsize{6pt}{6pt},
  }
\begin{lstlisting}[language=python]

def normalize(activations):
    activations = activations.unsqueeze(0)
    max_values = F.adaptive_max_pool2d(activations, (1, 1))
    min_values = -F.adaptive_max_pool2d(-activations, (1, 1))
    return (activations - min_values) / (max_values - min_values)

def calculate_iou(mask1, mask2, eps=1e-6):
    intersection = torch.sum(mask1 & mask2)
    union = torch.sum(mask1 | mask2)
    IoU = intersection / (union + eps)
    return IoU
		
def evaluate_comprehensiveness(model, test_dataset, threshold):
    all_IoUs = []
    for (image, ground_truth_foreground_map) in test_dataset:
        activations = model.get_activation(images) # shape: K, H, W
        activations = normalize(activations)
        activations_union = (activations >= threshold).sum(dim=0)
        IoU = calculate_IoU(
            activations_union,
            ground_truth_foreground_map
        )
        all_IoUs.append(IoU)
    return mean(all_IoUs)
\end{lstlisting}
\end{algorithm}

\section{Visualizations}
\label{sec:supp-visualizations}

We show the typical reasoning process of our framework across CUB-200-2011 in Table \ref{tab:supp-reasoning}. Each row displays how a particular prototype contributes to the logit of its corresponding class. Note that first column displays the prototype's most similar image patch from the training set, while the second column displays the source image of the prototype in the first column. In addition, we also provide more comparison of activation maps across ProtoPNet architectures in Figure \ref{fig:supp-comparison}.

\begin{figure*}[t]
  \centering
  \includegraphics[width=\textwidth]{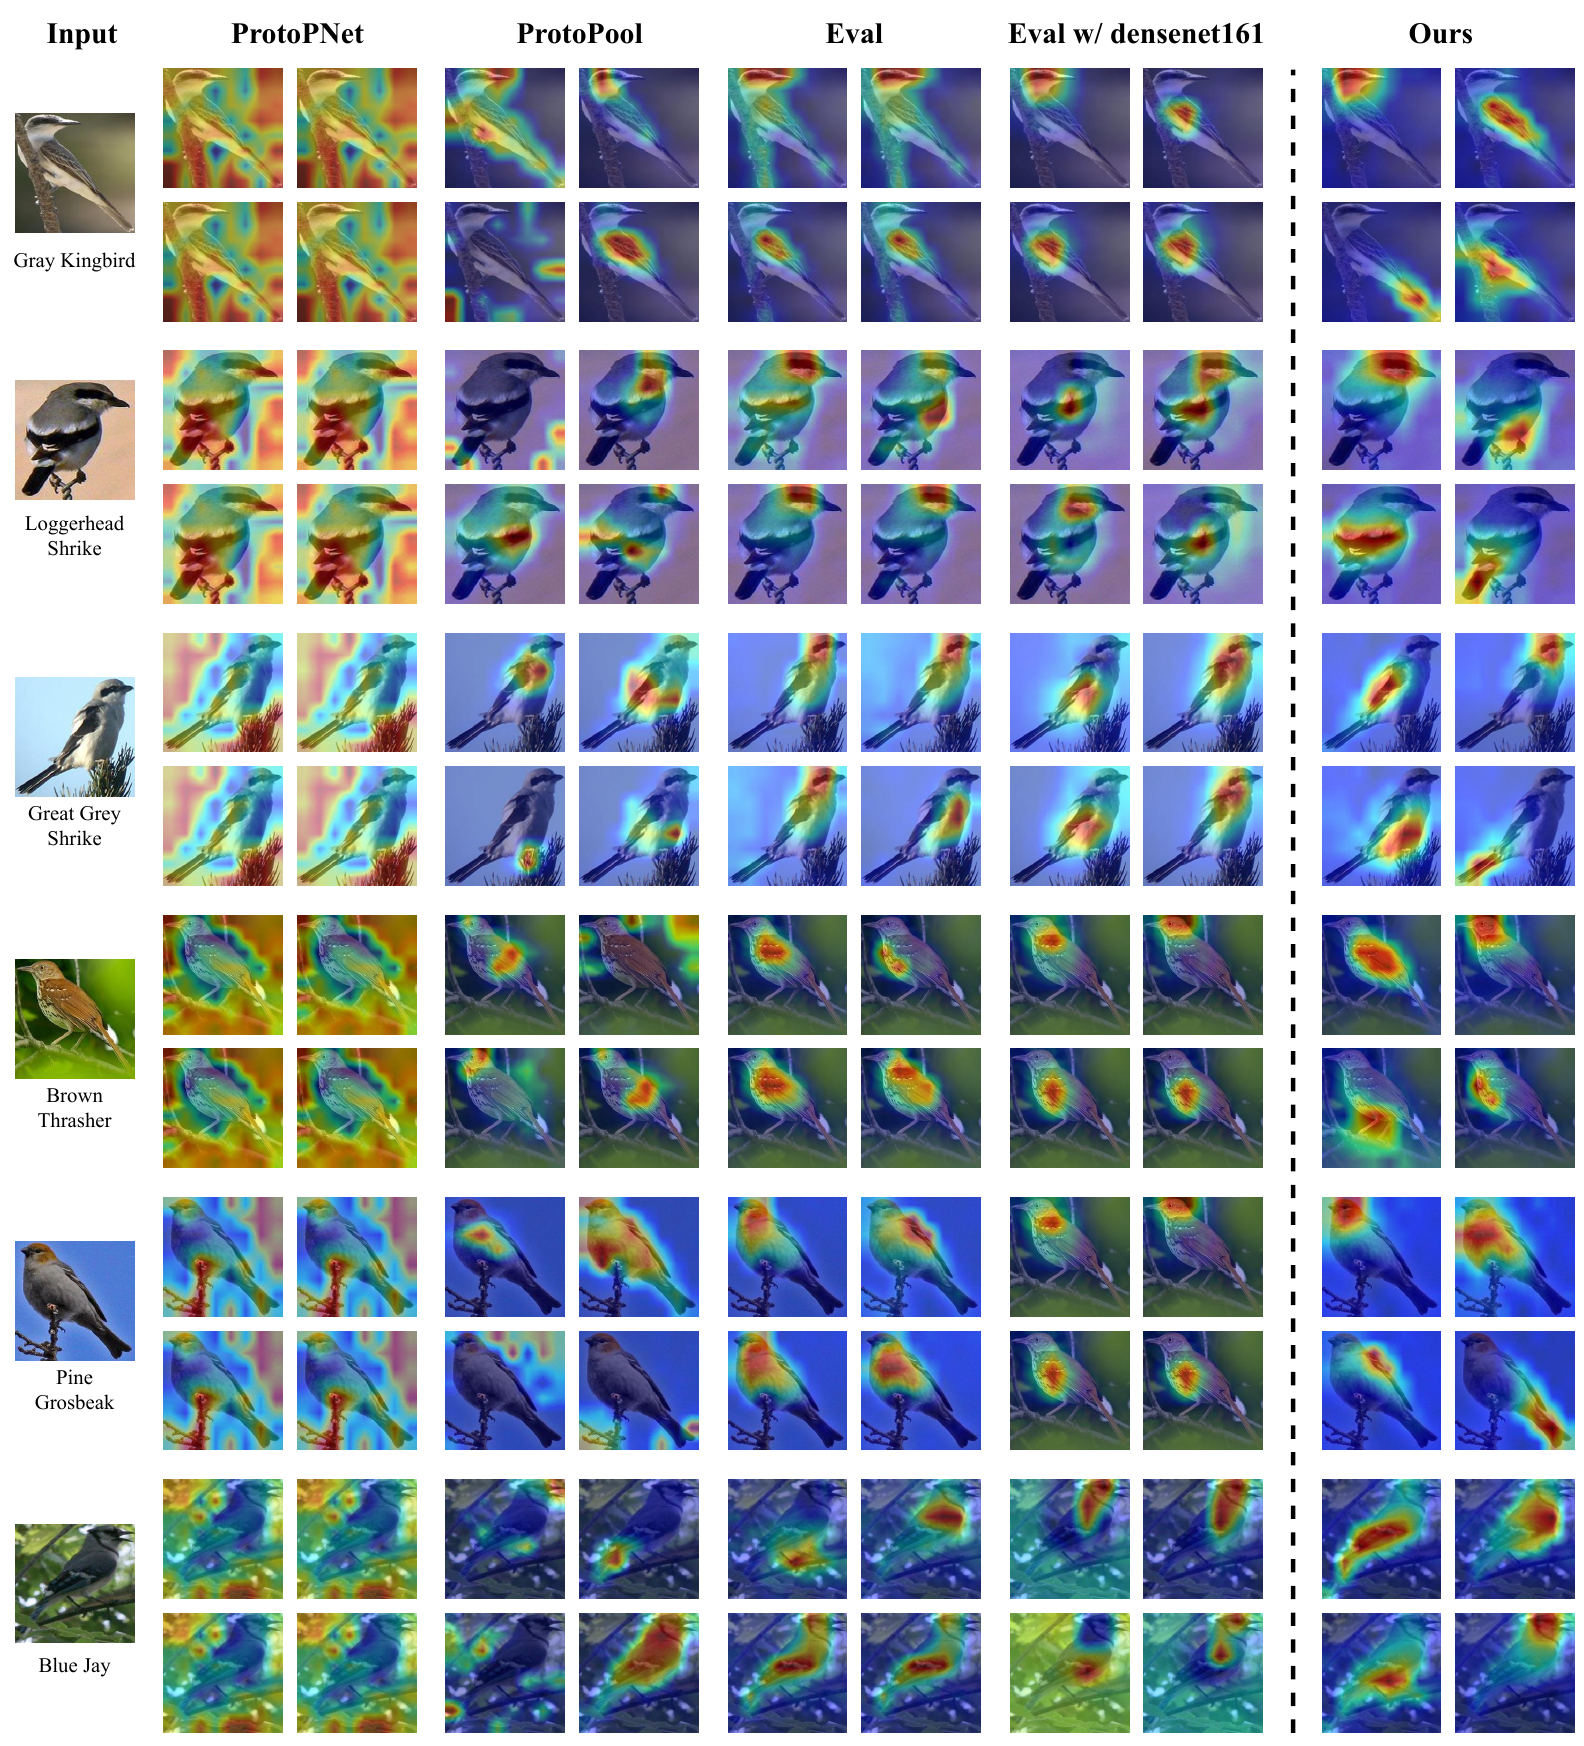}
  \caption[architecture]{Visualization on CUB-200-2011 test images across various ProtoPNet architectures. All models are trained using the same DINOv2 ViT-B backbone with $K=5$ unless annotated.}
  \label{fig:supp-comparison}
\end{figure*}

\newcolumntype{Y}{>{\centering\arraybackslash}X}
\newcolumntype{C}{>{\centering\let\newline\\\arraybackslash\hspace{0pt}}m{1cm}}
\newcommand{\myimg}[1]{\raisebox{-.5\height}{\includegraphics[width=0.18\columnwidth]{#1}}}
\newcommand{\myimgsmall}[1]{\raisebox{-0.0\height}{\includegraphics[scale=0.15]{#1}}}
\newcommand{\myimgmedium}[1]{\raisebox{-0.5\height}{\includegraphics[scale=0.3]{#1}}}

\begin{table*}
  \centering
  \begin{tabular}{cc}
    \resizebox{\columnwidth}{!}{
    \begin{tabularx}{\columnwidth}{Y Y Y C}
      \multicolumn{3}{l}{\makecell{\textbf{Why is this image classified as a} \\ \textbf{American Pipit ?}}} & \myimgsmall{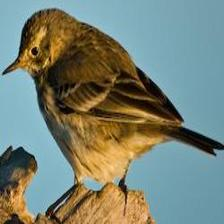} \\
      \\
      \toprule
      \textbf{Prototypical Part} & \textbf{Source Image} & \textbf{Activation Map} & \textbf{Score} \\
      \midrule
      \myimg{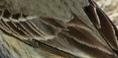} & \myimg{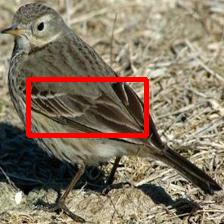} & \myimg{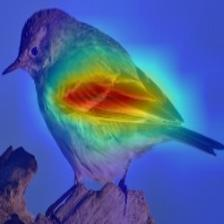} & 2.92 \\
      \\
      \myimg{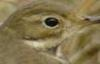} & \myimg{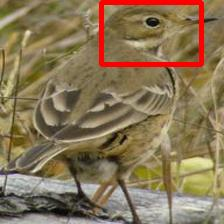} & \myimg{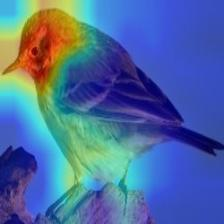} & 2.33 \\
      \\
      \myimg{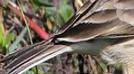} & \myimg{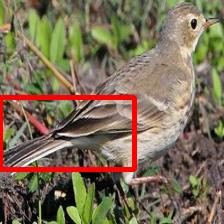} & \myimg{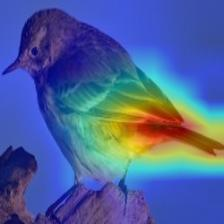} & 2.71 \\
      \\
      $\dots$ & $\dots$ & $\dots$ & $\dots$ \\
    \end{tabularx}
    } &
    \resizebox{\columnwidth}{!}{
    \begin{tabularx}{\columnwidth}{Y Y Y C}
      \multicolumn{3}{l}{\makecell{\textbf{Why is this image classified as a} \\ \textbf{Ringed Kingfisher ?}}} & \myimgsmall{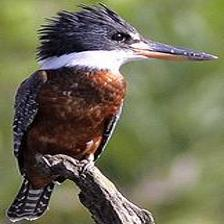} \\
      \\
      \toprule
      \textbf{Prototypical Part} & \textbf{Source Image} & \textbf{Activation Map} & \textbf{Score} \\
      \midrule
      \myimg{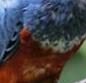} & \myimg{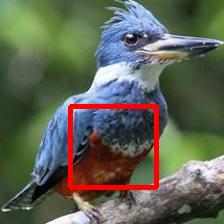} & \myimg{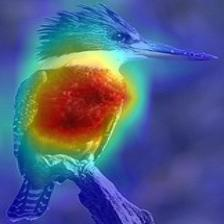} & 3.05 \\
      \\
      \myimg{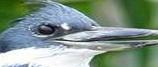} & \myimg{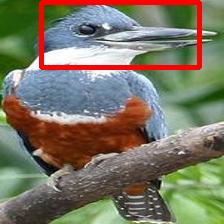} & \myimg{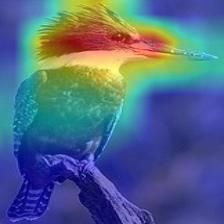} & 2.43 \\
      \\
      \myimg{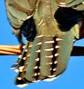} & \myimg{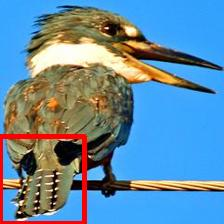} & \myimg{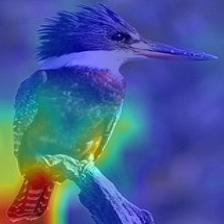} & 2.73 \\
      \\
      $\dots$ & $\dots$ & $\dots$ & $\dots$ \\
    \end{tabularx}
    } \\
    \resizebox{\columnwidth}{!}{
    \begin{tabularx}{\columnwidth}{Y Y Y C}
      \multicolumn{3}{l}{\makecell{\textbf{Why is this image classified as a} \\ \textbf{Western Grebe ?}}} & \myimgsmall{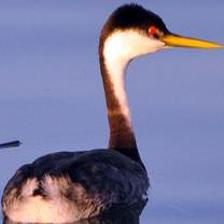} \\
      \\
      \toprule
      \textbf{Prototypical Part} & \textbf{Source Image} & \textbf{Activation Map} & \textbf{Score} \\
      \midrule
      \myimgmedium{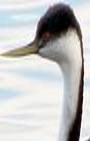} & \myimg{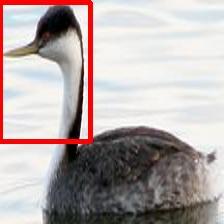} & \myimg{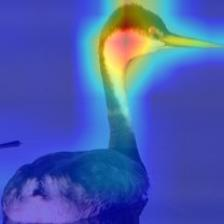} & 3.09 \\
      \\
      \myimgmedium{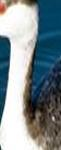} & \myimg{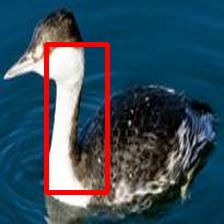} & \myimg{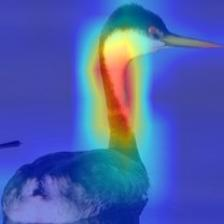} & 2.82 \\
      \\
      \myimgmedium{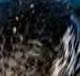} & \myimg{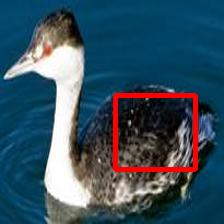} & \myimg{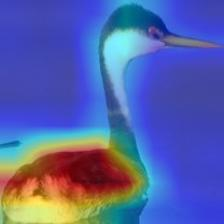} & 2.52 \\
      \\
      $\dots$ & $\dots$ & $\dots$ & $\dots$ \\
    \end{tabularx}
    } &
    \resizebox{\columnwidth}{!}{
    \begin{tabularx}{\columnwidth}{Y Y Y C}
      \multicolumn{3}{l}{\makecell{\textbf{Why is this image classified as a} \\ \textbf{Clark Nutcracker ?}}} & \myimgsmall{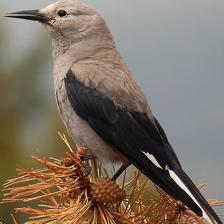} \\
      \\
      \toprule
      \textbf{Prototypical Part} & \textbf{Source Image} & \textbf{Activation Map} & \textbf{Score} \\
      \midrule
      \myimgmedium{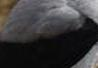} & \myimg{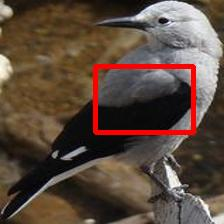} & \myimg{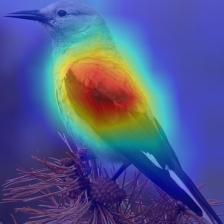} & 2.93 \\
      \\
      \myimgmedium{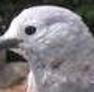} & \myimg{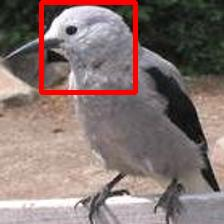} & \myimg{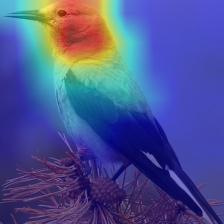} & 2.99 \\
      \\
      \myimgmedium{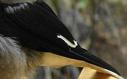} & \myimg{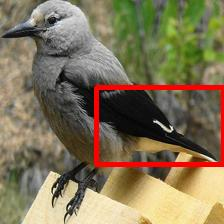} & \myimg{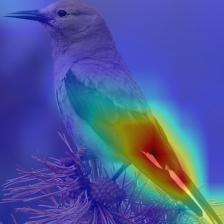} & 2.82 \\
      \\
      $\dots$ & $\dots$ & $\dots$ & $\dots$ \\
    \end{tabularx}
    } \\
    \resizebox{\columnwidth}{!}{
    \begin{tabularx}{\columnwidth}{Y Y Y C}
      \multicolumn{3}{l}{\makecell{\textbf{Why is this image classified as a} \\ \textbf{Great Grey Shrike ?}}} & \myimgsmall{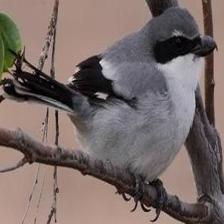} \\
      \\
      \toprule
      \textbf{Prototypical Part} & \textbf{Source Image} & \textbf{Activation Map} & \textbf{Score} \\
      \midrule
      \myimgmedium{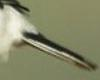} & \myimg{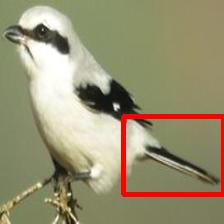} & \myimg{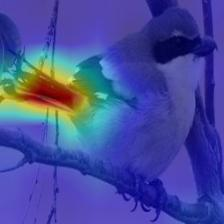} & 2.99 \\
      \\
      \myimgmedium{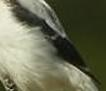} & \myimg{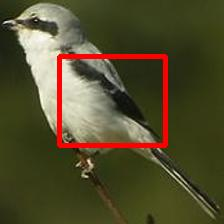} & \myimg{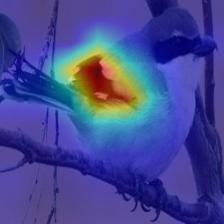} & 3.02 \\
      \\
      \myimgmedium{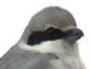} & \myimg{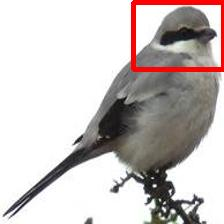} & \myimg{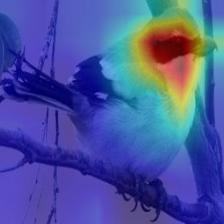} & 3.28 \\
      \\
      $\dots$ & $\dots$ & $\dots$ & $\dots$ \\
    \end{tabularx}
    } &
    \resizebox{\columnwidth}{!}{
    \begin{tabularx}{\columnwidth}{Y Y Y C}
      \multicolumn{3}{l}{\makecell{\textbf{Why is this image classified as a} \\ \textbf{Yellow Warbler ?}}} & \myimgsmall{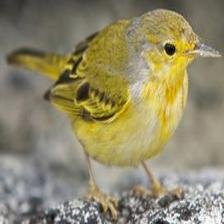} \\
      \\
      \toprule
      \textbf{Prototypical Part} & \textbf{Source Image} & \textbf{Activation Map} & \textbf{Score} \\
      \midrule
      \myimgmedium{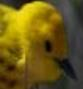} & \myimg{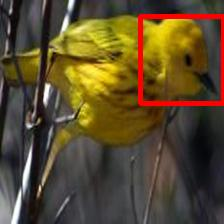} & \myimg{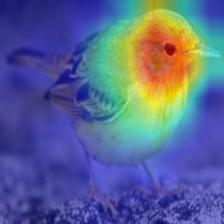} & 2.88 \\
      \\
      \myimgmedium{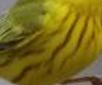} & \myimg{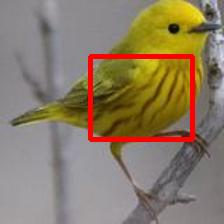} & \myimg{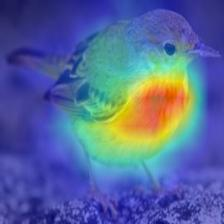} & 2.73 \\
      \\
      \myimgmedium{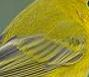} & \myimg{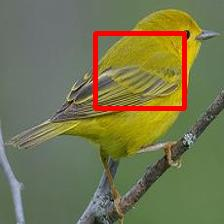} & \myimg{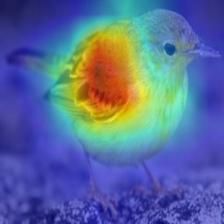} & 3.26 \\
      \\
      $\dots$ & $\dots$ & $\dots$ & $\dots$ \\
    \end{tabularx}
    }
  \end{tabular}
  \caption{Visualization of the typical visual reasoning process of our framework on CUB-200-2011 dataset.}
  \label{tab:supp-reasoning}
\end{table*}

\clearpage

%%% Local Variables:
%%% mode: latex
%%% TeX-master: "../main.tex"
%%% reftex-default-bibliography: ("../main.bib") ***
%%% End:
