# Supplementary material for: Interpretable Image Classification via Non-parametric Part Prototype Learning
Source: arXiv:2503.10247 source file (2025-03-13)
Supplement: Supplementary file 2 [file supp_reasoning_visualization.tex]

\newcolumntype{Y}{>{\centering\arraybackslash}X}
\newcolumntype{C}{>{\centering\let\newline\\\arraybackslash\hspace{0pt}}m{1cm}}
\newcommand{\myimg}[1]{\raisebox{-.5\height}{\includegraphics[width=0.18\columnwidth]{#1}}}
\newcommand{\myimgsmall}[1]{\raisebox{-0.0\height}{\includegraphics[scale=0.15]{#1}}}
\newcommand{\myimgmedium}[1]{\raisebox{-0.5\height}{\includegraphics[scale=0.3]{#1}}}

\begin{table*}
  \centering
  \begin{tabular}{cc}
    \resizebox{\columnwidth}{!}{
    \begin{tabularx}{\columnwidth}{Y Y Y C}
      \multicolumn{3}{l}{\makecell{\textbf{Why is this image classified as a} \\ \textbf{American Pipit ?}}} & \myimgsmall{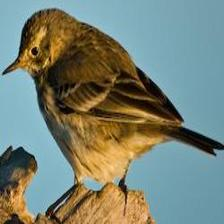} \\
      \\
      \toprule
      \textbf{Prototypical Part} & \textbf{Source Image} & \textbf{Activation Map} & \textbf{Score} \\
      \midrule
      \myimg{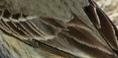} & \myimg{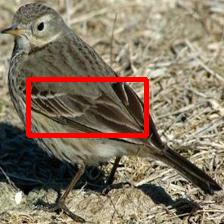} & \myimg{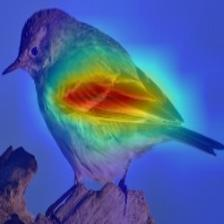} & 2.92 \\
      \\
      \myimg{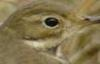} & \myimg{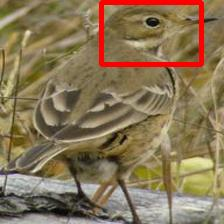} & \myimg{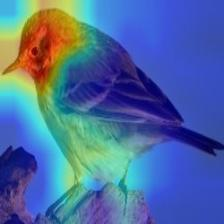} & 2.33 \\
      \\
      \myimg{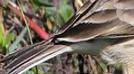} & \myimg{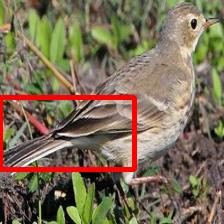} & \myimg{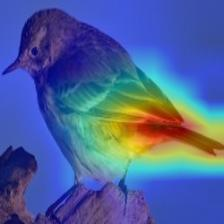} & 2.71 \\
      \\
      $\dots$ & $\dots$ & $\dots$ & $\dots$ \\
    \end{tabularx}
    } &
    \resizebox{\columnwidth}{!}{
    \begin{tabularx}{\columnwidth}{Y Y Y C}
      \multicolumn{3}{l}{\makecell{\textbf{Why is this image classified as a} \\ \textbf{Ringed Kingfisher ?}}} & \myimgsmall{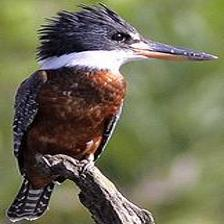} \\
      \\
      \toprule
      \textbf{Prototypical Part} & \textbf{Source Image} & \textbf{Activation Map} & \textbf{Score} \\
      \midrule
      \myimg{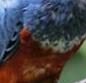} & \myimg{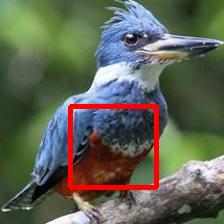} & \myimg{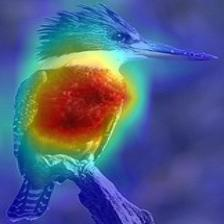} & 3.05 \\
      \\
      \myimg{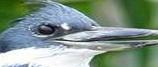} & \myimg{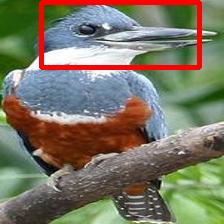} & \myimg{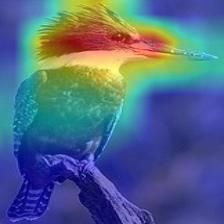} & 2.43 \\
      \\
      \myimg{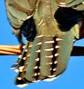} & \myimg{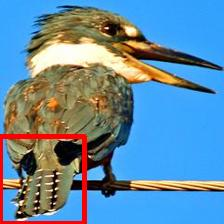} & \myimg{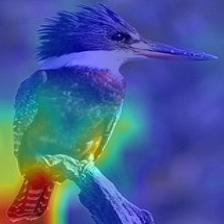} & 2.73 \\
      \\
      $\dots$ & $\dots$ & $\dots$ & $\dots$ \\
    \end{tabularx}
    } \\
    \resizebox{\columnwidth}{!}{
    \begin{tabularx}{\columnwidth}{Y Y Y C}
      \multicolumn{3}{l}{\makecell{\textbf{Why is this image classified as a} \\ \textbf{Western Grebe ?}}} & \myimgsmall{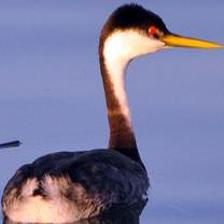} \\
      \\
      \toprule
      \textbf{Prototypical Part} & \textbf{Source Image} & \textbf{Activation Map} & \textbf{Score} \\
      \midrule
      \myimgmedium{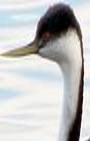} & \myimg{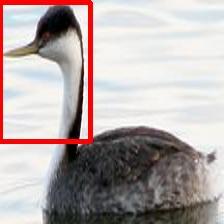} & \myimg{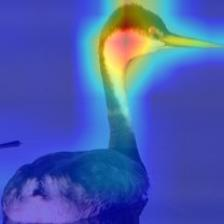} & 3.09 \\
      \\
      \myimgmedium{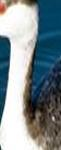} & \myimg{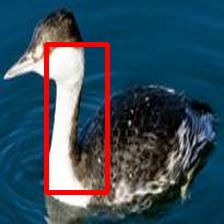} & \myimg{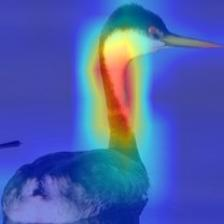} & 2.82 \\
      \\
      \myimgmedium{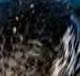} & \myimg{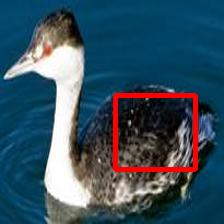} & \myimg{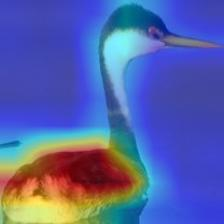} & 2.52 \\
      \\
      $\dots$ & $\dots$ & $\dots$ & $\dots$ \\
    \end{tabularx}
    } &
    \resizebox{\columnwidth}{!}{
    \begin{tabularx}{\columnwidth}{Y Y Y C}
      \multicolumn{3}{l}{\makecell{\textbf{Why is this image classified as a} \\ \textbf{Clark Nutcracker ?}}} & \myimgsmall{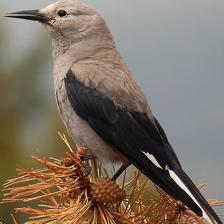} \\
      \\
      \toprule
      \textbf{Prototypical Part} & \textbf{Source Image} & \textbf{Activation Map} & \textbf{Score} \\
      \midrule
      \myimgmedium{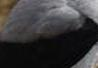} & \myimg{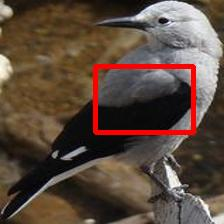} & \myimg{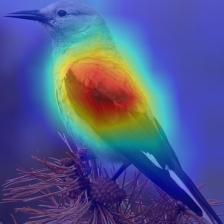} & 2.93 \\
      \\
      \myimgmedium{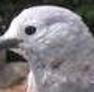} & \myimg{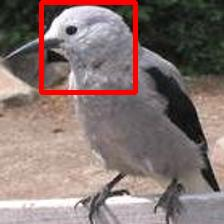} & \myimg{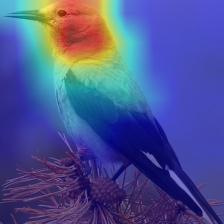} & 2.99 \\
      \\
      \myimgmedium{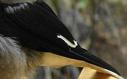} & \myimg{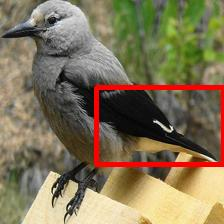} & \myimg{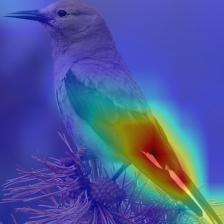} & 2.82 \\
      \\
      $\dots$ & $\dots$ & $\dots$ & $\dots$ \\
    \end{tabularx}
    } \\
    \resizebox{\columnwidth}{!}{
    \begin{tabularx}{\columnwidth}{Y Y Y C}
      \multicolumn{3}{l}{\makecell{\textbf{Why is this image classified as a} \\ \textbf{Great Grey Shrike ?}}} & \myimgsmall{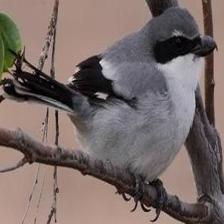} \\
      \\
      \toprule
      \textbf{Prototypical Part} & \textbf{Source Image} & \textbf{Activation Map} & \textbf{Score} \\
      \midrule
      \myimgmedium{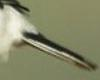} & \myimg{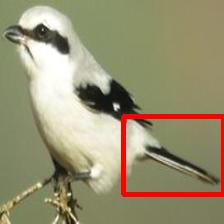} & \myimg{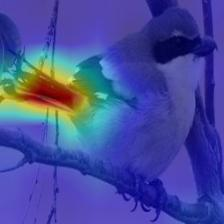} & 2.99 \\
      \\
      \myimgmedium{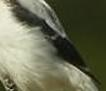} & \myimg{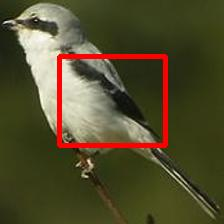} & \myimg{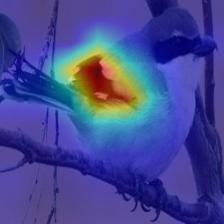} & 3.02 \\
      \\
      \myimgmedium{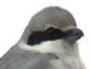} & \myimg{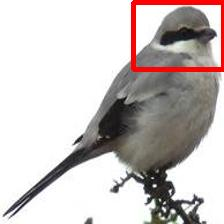} & \myimg{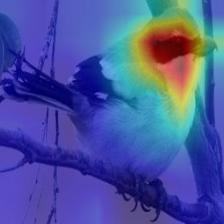} & 3.28 \\
      \\
      $\dots$ & $\dots$ & $\dots$ & $\dots$ \\
    \end{tabularx}
    } &
    \resizebox{\columnwidth}{!}{
    \begin{tabularx}{\columnwidth}{Y Y Y C}
      \multicolumn{3}{l}{\makecell{\textbf{Why is this image classified as a} \\ \textbf{Yellow Warbler ?}}} & \myimgsmall{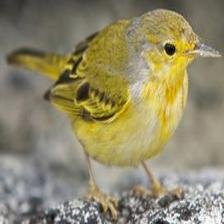} \\
      \\
      \toprule
      \textbf{Prototypical Part} & \textbf{Source Image} & \textbf{Activation Map} & \textbf{Score} \\
      \midrule
      \myimgmedium{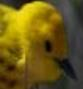} & \myimg{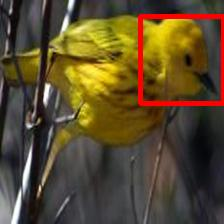} & \myimg{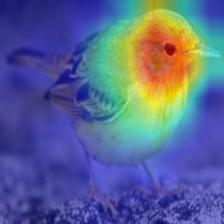} & 2.88 \\
      \\
      \myimgmedium{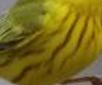} & \myimg{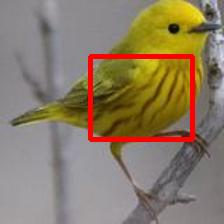} & \myimg{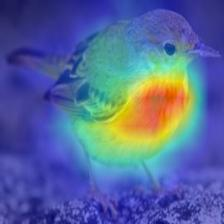} & 2.73 \\
      \\
      \myimgmedium{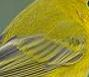} & \myimg{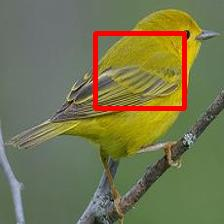} & \myimg{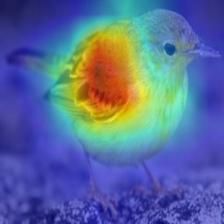} & 3.26 \\
      \\
      $\dots$ & $\dots$ & $\dots$ & $\dots$ \\
    \end{tabularx}
    }
  \end{tabular}
  \caption{Visualization of the typical visual reasoning process of our framework on CUB-200-2011 dataset.}
  \label{tab:supp-reasoning}
\end{table*}
