# Supplementary material for: Interpretable Image Classification via Non-parametric Part Prototype Learning
Source: arXiv:2503.10247 source file (2025-03-13)
Supplement: Supplementary file 3 [file supp_algo.tex]

\begin{algorithm}
\caption{Prototype Learning and Backbone Fine-tuning}
\label{alg:training}
\begin{algorithmic}[1]
  \Require Training set $\mathcal{X}$, $nEpochs$, ViT backbone $\mathcal{F}$
\State Initialize prototypes $\mathbf{P}$ and modulation vector $w$ with $\mathbf{P} \sim \mathcal{N}(0.0, 0.02)$ and $w^c_k=0.2$
\For{$t \in \{1, \dots, nEpochs\}$}
    \State Randomly split $\mathcal{X}$ into mini-batches
    \For{$(\mathbf{X}, \mathbf{y}) \in \{\mathcal{X}_1, \dots\}$}
        \State $\mathbf{f} = \text{reshape}(\mathcal{F}(\mathbf{X})) \in \mathbb{R}^{Bhw \times D}$
        \State $\mathcal{M} = \phi(\mathbf{f}, \mathbf{X}) \in \{0, 1\}^{Bhw}$
        \State $\mathbf{S} = \text{reshape}(\text{Sim}(\mathbf{f}, \mathbf{P})) \in \mathbb{R}^{Bhw \times N \times K}$
        \For{$c \in \text{unique}(\mathbf{y})$}
          \State Get $\mathbf{S}^c$ and $\mathbf{f}^c$ by indexing $\mathbf{S}$, $\mathbf{f}$ with $\mathcal{M}$, $\mathbf{y}$
          \State $\mathbf{A}^{c,*} = \text{sinkhorn\_knopp}(\mathbf{S}^c)$
          \If{\textit{first training stage}}
            \State $\mathbf{P}^c \leftarrow \beta \mathbf{P}^c + (1 - \beta) (\mathbf{A}^{c,*})^\top\mathbf{f}^c$
          \EndIf
        \EndFor
        \State $g = \text{MaxPool}(\text{reshape}(\mathbf{S})) \in \mathbb{R}^{N \times K}$
        \State $\text{logits} = \text{compute\_logits}(g, w) \in \mathbb{R}^N$
        \If{\textit{second training stage}}
          \State Compute loss $\mathcal{L}_{xe}(\text{logits}, \mathbf{y})$
          \State Compute loss $\mathcal{L}_{PPC}(\mathbf{S}, \mathbf{A})$
          \State Minimize loss by updating $\mathcal{F}$
        \EndIf
    \EndFor
\EndFor
\end{algorithmic}
\end{algorithm}
