# Supplementary material for: Interpretable Image Classification via Non-parametric Part Prototype Learning
Source: arXiv:2503.10247 source file (2025-03-13)
Supplement: Supplementary file 4 [file supp_compre_algo.tex]

\begin{algorithm}[t]
  \caption{Python-like pseudo-code of Comprehensiveness Score calculation.}
  \label{alg:compre}
  \definecolor{codeblue}{rgb}{0.25,0.5,0.5}
  \lstset{
    backgroundcolor=\color{white},
    basicstyle=\fontsize{6pt}{6pt}\ttfamily\selectfont,
    columns=fullflexible,
    breaklines=true,
    captionpos=b,
    commentstyle=\fontsize{6pt}{6pt}\color{codeblue},
    keywordstyle=\fontsize{6pt}{6pt},
  }
\begin{lstlisting}[language=python]

def normalize(activations):
    activations = activations.unsqueeze(0)
    max_values = F.adaptive_max_pool2d(activations, (1, 1))
    min_values = -F.adaptive_max_pool2d(-activations, (1, 1))
    return (activations - min_values) / (max_values - min_values)

def calculate_iou(mask1, mask2, eps=1e-6):
    intersection = torch.sum(mask1 & mask2)
    union = torch.sum(mask1 | mask2)
    IoU = intersection / (union + eps)
    return IoU
		
def evaluate_comprehensiveness(model, test_dataset, threshold):
    all_IoUs = []
    for (image, ground_truth_foreground_map) in test_dataset:
        activations = model.get_activation(images) # shape: K, H, W
        activations = normalize(activations)
        activations_union = (activations >= threshold).sum(dim=0)
        IoU = calculate_IoU(
            activations_union,
            ground_truth_foreground_map
        )
        all_IoUs.append(IoU)
    return mean(all_IoUs)
\end{lstlisting}
\end{algorithm}
