# Supplementary material for: Interpretable Image Classification via Non-parametric Part Prototype Learning
Source: arXiv:2503.10247 source file (2025-03-13)
Supplement: Supplementary file 5 [file supp_distinc_algo.tex]

\begin{algorithm}[t]
  \caption{Python-like pseudo-code of Distinctiveness Score calculation.}
  \label{alg:distinctiveness}
  \definecolor{codeblue}{rgb}{0.25,0.5,0.5}
  \lstset{
    backgroundcolor=\color{white},
    basicstyle=\fontsize{6pt}{6pt}\ttfamily\selectfont,
    columns=fullflexible,
    breaklines=true,
    captionpos=b,
    commentstyle=\fontsize{6pt}{6pt}\color{codeblue},
    keywordstyle=\fontsize{6pt}{6pt},
  }
\begin{lstlisting}[language=python]
def evaluate_distinctiveness(model, test_dataset, bbox_size):
    all_O_x = []
    for image in test_dataset:
        activations = model.get_activation(images) # shape: K, H, W
        sample_IoUs = []
        for i in range(K):
            for j in range(K):
                activation_i_max_coord = max_coord(activations[i])
                activation_j_max_coord = max_coord(activations[j])
                bbox_i = get_bbox(activation_i_max_coord)
                bbox_j = get_bbox(activation_j_max_coord)
                IoU = compute_box_IoU(bbox_i, bbox_j)
                sample_IoUs.append(IoU)
        O_x = mean(sample_IoUs)
        all_O_x.append(O_x)
    return 1 - mean(all_O_x)
\end{lstlisting}
\end{algorithm}
