# Supplementary material for: Interpretable Image Classification via Non-parametric Part Prototype Learning
Source: arXiv:2503.10247 source file (2025-03-13)
Supplement: Supplementary file 6 [file supp_cars_results.tex]

\newcolumntype{Y}{>{\centering\arraybackslash}X}

\begin{table}
  \centering
  \resizebox{0.95\columnwidth}{!}{
  \begin{tabularx}{\columnwidth}{c|Y|Y}
    \toprule
      \textbf{Methods} & \textbf{ViT-B} & \textbf{ViT-S} \\
      \midrule
      ProtoPNet (K=3) & 86.47 & 78.16 \\
      ProtoPNet (K=5) & 86.75 & 79.51 \\
      \hline
      TesNet (K=3) & 87.33 & 80.97 \\
      TesNet (K=5) & 87.15 & 82.55 \\
      \hline
      EvalProtoPNet & 91.20 & 83.40 \\
      EvalProtoPNet & 91.46 & \textbf{87.09} \\
      \hline
      Ours (K=3) & 91.29 & 85.52 \\
      Ours (K=5) & \textbf{93.63} & 86.10 \\
      \bottomrule
    \end{tabularx}
  }
  \caption{Classification results on Stanford Cars dataset. All methods are trained with DINOv2. Best results are in bold.}
  \label{tab:supp-cars-results}
\end{table}
