# Supplementary material for: Interpretable Image Classification via Non-parametric Part Prototype Learning
Source: arXiv:2503.10247 source file (2025-03-13)
Supplement: Supplementary file 7 [file supp_dogs_results.tex]

\newcolumntype{Y}{>{\centering\arraybackslash}X}

\begin{table}
  \centering
  \resizebox{0.95\columnwidth}{!}{
  \begin{tabularx}{\columnwidth}{c|Y|Y}
    \toprule
      \textbf{Methods} & \textbf{ViT-B} & \textbf{ViT-S} \\
      \midrule
      ProtoPNet (K=3) & 84.11 & 79.25 \\
      ProtoPNet (K=5) & 84.90 & 79.28 \\
      \hline
      TesNet (K=3) & 85.16 & 82.14 \\
      TesNet (K=5) & 87.44 & 82.01 \\
      \hline
      EvalProtoPNet & 87.88 & 83.68 \\
      EvalProtoPNet & 88.08 & 83.80 \\
      \hline
      Ours (K=3) & 87.05 & 83.11 \\
      Ours (K=5) & \textbf{88.59} & \textbf{83.93} \\
      \bottomrule
    \end{tabularx}
  }
  \caption{Classification results on Stanford Dogs dataset. All methods are trained with DINOv2. Best results are in bold.}
  \label{tab:supp-dogs-results}
\end{table}
