# Supplementary material for: Interpretable Image Classification via Non-parametric Part Prototype Learning
Source: arXiv:2503.10247 source file (2025-03-13)
Supplement: Supplementary file 8 [file supp_fg_extraction_ablation.tex]

\begin{table}[b]
  \centering
  \resizebox{\columnwidth}{!}{
    \begin{tabular}{lcccc}
      \toprule
      & Con. & Sta. & Dis. & Class. \\
      \hline
      No foreground extraction & 29.67 & 82.85 & 94.17 & 88.42 \\
      PaPr w/ resnet18 & 51.01 & 82.33 & 97.23 & 88.76 \\
      Attention Rollout & 61.90 & 79.97 & 92.77 & 90.75 \\
      First Principal Component & \textbf{66.40} & \textbf{82.97} & \textbf{94.45} & \textbf{90.82} \\
      \bottomrule
    \end{tabular}
  }
  \caption{The effect of various off-the-shelf ViT foreground patch extraction methods on the performance of our framework.}
  \label{tab:ablation-fg-extraction}
\end{table}
